# Supplementary material for: The StarCraft Multi-Agent Challenge
Source: arXiv:1902.04043 source file (2019-12-09)
Supplement: Supplementary file 1 [file graphs.tex]

\section{Full Results}\label{appendix:results}

\newcommand{\gw}{0.329}

The median test win rates during the training of QMIX, COMA, and IQL methods on easy, hard and super hard SMAC scenarios are presented in Figures \ref{table:easy}, \ref{table:hard}, and \ref{table:super_hard}, respectively. All experiments feature 12 independent runs.

\begin{figure*}[htb!]
	\centering
	\includegraphics[height=0.35cm]{figures/all_graphs/base_legend}
	\vfill
	\includegraphics[width=\gw\textwidth]{figures/all_graphs/3m}
	\includegraphics[width=\gw\textwidth]{figures/all_graphs/8m}
	\includegraphics[width=\gw\textwidth]{figures/all_graphs/2s3z}\\
	\includegraphics[width=\gw\textwidth]{figures/all_graphs/MMM}
	\includegraphics[width=\gw\textwidth]{figures/all_graphs/micro_2M_Z}
	\includegraphics[width=\gw\textwidth]{figures/all_graphs/micro_retarget}\\
	\includegraphics[width=\gw\textwidth]{figures/all_graphs/3s_vs_3z}
	\includegraphics[width=\gw\textwidth]{figures/all_graphs/3s_vs_4z}
	\includegraphics[width=\gw\textwidth]{figures/all_graphs/micro_bane}\\
	\includegraphics[width=\gw\textwidth]{figures/all_graphs/micro_baneling}
	\caption{Median win rates for QMIX, COMA, and IQL on easy SMAC scenarios. 25\%-75\% percentile is shaded.}
	\label{table:easy}
\end{figure*}

\begin{figure*}[htb!]
	\centering
	\includegraphics[height=0.35cm]{figures/all_graphs/base_legend}
	\vfill
	\includegraphics[width=\gw\textwidth]{figures/all_graphs/25m}
	\includegraphics[width=\gw\textwidth]{figures/all_graphs/3s5z}
	\includegraphics[width=\gw\textwidth]{figures/all_graphs/5m_6m}\\
	\includegraphics[width=\gw\textwidth]{figures/all_graphs/8m_9m}
	\includegraphics[width=\gw\textwidth]{figures/all_graphs/10m_11m}
	\includegraphics[width=\gw\textwidth]{figures/all_graphs/3s_vs_5z}\\
	\includegraphics[width=\gw\textwidth]{figures/all_graphs/micro_colossus}
	\caption{Median win rates for QMIX, COMA, and IQL on hard SMAC scenarios. 25\%-75\% percentile is shaded.} 
	\label{table:hard}
\end{figure*}

\begin{figure*}[htb!]
	\centering
	\includegraphics[height=0.35cm]{figures/all_graphs/base_legend}
	\vfill
	\includegraphics[width=\gw\textwidth]{figures/all_graphs/27m_30m}
	\includegraphics[width=\gw\textwidth]{figures/all_graphs/3s5z_3s6z}
	\includegraphics[width=\gw\textwidth]{figures/all_graphs/MMM2}
	\includegraphics[width=\gw\textwidth]{figures/all_graphs/micro_focus}
	\includegraphics[width=\gw\textwidth]{figures/all_graphs/micro_corridor}
	\caption{Median win rates for QMIX, COMA, and IQL on super hard SMAC scenarios. 25\%-75\% percentile is shaded.} 
	\label{table:super_hard}
\end{figure*}
