# Supplementary material for: The StarCraft Multi-Agent Challenge
Source: arXiv:1902.04043 source file (2019-12-09)
Supplement: Supplementary file 2 [file result_discussion.tex]

\section{Results Discussion}\label{appendix:discussion}

In this section, we present the results of running our chosen agents across the scenarios, and offer some discussion of the learnt policies we have observed. Finally, we investigate the necessity of using an RNN in our agent networks to tackle partial observability.

Based on these results in Table \ref{tab:results_all}, we broadly categorise the scenarios into three categories for our discussion below: \textit{Easy}, \textit{Hard}, and \textit{Super Hard}. The \textit{Easy} scenarios are fully solved (above $95\%$ median win rate) by our QMIX setup within the timeframe given, whereas we make progress on but do not solve the \textit{Hard} scenarios. The \textit{Super Hard} scenarios are perhaps the most interesting since our QMIX agent makes little to no progress on them. 

\subsection{Easy scenarios}

The symmetric scenarios generally provide an easier challenge to learning agents. The enemy utilises a fixed strategy and possesses no advantage in unit composition or number compared to the allied team, which allows the team of learning agents to develop a strategy to win in almost every encounter.

The \texttt{3m} scenario provides the easiest challenge of all the scenarios, and is fully solved by both IQL and QMIX. It is an ideal scenario to debug algorithm implementations and investigate hyperparameter configurations on, serving a similar role to Pong in the ALE. 
The \texttt{8m} scenario  provides a larger challenge, owing mainly to the increased number of agents that must learn to coordinate when focussing fire. Our QMIX agents were able to learn to first position into a line, in order to ensure that they can all begin attacking at the same time and to focus fire without overkill. They also learned to run back from the attack line upon absorbing severe hit-point damage. COMA and IQL agents also learned to win the \texttt{8m} scenario most of the time, although the cooperation between agents is less coordinated compared with QMIX.

\begin{figure}
	\centering
	\subfigure[]{
		\includegraphics[width=0.49\linewidth]{figures/graphs/MMM_test_battle_won_mean_median.png}}
	\subfigure[]{
		\includegraphics[width=0.49\linewidth]{figures/graphs/3s_vs_345z_test_battle_won_mean_median.png}}
	\captionof{figure}{Median win rate of (a) QMIX, COMA, and IQL on \texttt{MMM} scenario and (b) QMIX on \texttt{3s\_vs\_3z}, \texttt{3s\_vs\_4z} and \texttt{3s\_vs\_5z} scenarios. 25\%-75\% percentile is shaded.}
	\label{fig:MMM_and_3svs345z_graph}
\end{figure}

The \texttt{MMM} and \texttt{2s3z} scenarios prove harder, but are still solvable by QMIX within the training period. Notably, we begin to see a large disparity between QMIX and both IQL and COMA on these scenarios. Figure \ref{fig:MMM_and_3svs345z_graph}a shows the performance of the 3 methods across the training. Our QMIX agents are able to learn the strategy of focus fire and protecting the Medivac from damage on the \texttt{MMM} scenario, whereas IQL and COMA do not. On the \texttt{2s3z} scenario QMIX successfully learned to intercept the enemy Zealots with allied Zealots in order to protect the allied Stalkers from severe damage which requires deliberate movement.

On the \texttt{2m\_vs\_1z} scenario we can see that both IQL and QMIX are able to fully solve it, which requires the 2 Marines to alternately fire on the enemy Zealot in order to draw its attention away from the other allied Marine. COMA, on the other hand does not learn to draw the enemy Zealot away from the Marines, and thus takes heavy damage and loses the scenario in the vast majority of cases. \texttt{2m\_vs\_1z}, which is a similar scenario where 2 allied Stalkers face a Spine Crawler, is also solved by QMIX and IQL. Here, the agents learned to make the enemy retarget once any of the Stalkers absorbs severe hit-point damage in order not to get killed.

The \texttt{so\_many\_banelings} scenario requires the agents to sacrifice themselves to the enemy Banelings. The optimal strategy is to spread out in order to both minimise the number of allied units which are damaged and maximise the number of enemy Banelings which are hit within the damage radius. %
The QMIX agents learn this winning strategy, whereas the COMA and IQL agents do not spread out enough and take unnecessary damage leading to an unstable and mediocre win rate.

Banelings also play a key role in the \texttt{bane\_vs\_bane} scenario. Here, QMIX and IQL agents were able to learn a winning strategy in which the allied Banelings attack the enemy first to deal severe damage, only after which Zerglings start to attack. COMA agents were not able to coordinate well in order to master such a winning strategy. 

An optimal strategy for the \texttt{3s\_vs\_3z}, \texttt{3s\_vs\_4z}, and \texttt{3s\_vs\_5z} scenarios is to kite the enemy Zealots. On the \texttt{3s\_vs\_3z} scenario only QMIX is able to learn such a strategy. A similar strategy is learnt by QMIX for the \texttt{3s\_vs\_4z} scenario, but only the best runs are able to solve it within the training period indicating that the learning speed of our algorithm is the main bottleneck here. 

\subsection{Hard scenarios}

Despite having the same number of Marines on both side, the \texttt{25m} scenario is much harder compared with \texttt{3m} and \texttt{8m}. Defeating the enemy here requires a higher-level of coordination when focussing fire, which is difficult when the number of independent agents is large. None of the methods were able to learn a consistently winning strategy.

Unlike the \texttt{3s\_vs\_3z} and \texttt{3s\_vs\_4z} scenarios, the QMIX agents are unable to solve the \texttt{3s\_vs\_5z} scenario within the training period. A look at the learned policies shows better kiting in some situations compared to \texttt{3s\_vs\_4z}, but overall worse performance. We hypothesise that the longer episodes make it more difficult to train, since temporal credit assignment is harder. This further highlights the need for faster training. Figure \ref{fig:MMM_and_3svs345z_graph}b shows the performance of the QMIX agents across the 3 scenarios.

Compared to its easier counterpart, \texttt{3s5z} is a much harder scenario. The learnt strategies for the best QMIX agents are very different compared to the best strategies learnt for \texttt{2s3z}. In this scenario the QMIX Zealots do not purposefully intercept the enemy Zealots, and thus the allied Stalkers die very quickly leading to a guaranteed loss. We have observed that a longer training period does indeed lead to much better performance on this scenario. %
We hypothesise that a better exploration scheme would help in this regard, since the agents would be exposed to better strategies more often, as opposed to requiring many training iterations and some luck to discover a better positioning for their units. 

The asymmetric scenarios \texttt{5m\_vs\_6m}, \texttt{8m\_vs\_9m}, and \texttt{10m\_vs\_11m} offer a substantial challenge. The allied agents must learn to focus fire without overkill and to correctly position themselves with considerable precision. The QMIX agents make good progress, but are unable to learn to both focus fire appropriately and position themselves correctly before encountering the enemy. This is particularly prevalent on the \texttt{10m\_vs\_11m} scenario, where a number of the allied agents are still positioning themselves when the enemy is encountered. The lack of a performance hit despite this is due to the easier nature of the \texttt{10m\_11m} scenario compared to \texttt{5m\_vs\_6m} owing to the relative army sizes. 

The difficulty of the \texttt{2c\_vs\_64zg} scenario lies in the number of enemy units, which makes the action space of the agents much larger than in other scenarios. The allied Colossi need to make use of the cliff to buy time and kill as many Zerglings as possible before can they reach them from all sides. Our QMIX agents learned to make use of this terrain feature but were unable to fully master this scenario. 

\subsection{Super Hard scenarios}

Of the 22 scenarios featured in initial release of SMAC, our QMIX agent makes very little progress on 5 of them: \texttt{27m\_vs\_30m}, \texttt{3s5z\_vs\_3s6z}, \texttt{MMM2}, \texttt{6h\_vs\_8z} and \texttt{corridor}.

\texttt{corridor} presents a task in which active state space exploration is required. An optimal strategy for this scenario requires the allied Zealots to move to a choke point on the map, so as to not be surrounded by the enemy army. None of our tested methods utilise any form of directed state space exploration, which leads to them all remaining in the local optimum of merely damaging the enemy units for reward, instead of first moving to the choke point and then attacking.  

The hardest of all Marine scenarios is \texttt{27m\_vs\_30m} on which all three methods make little to no progress. Only the QMIX agents were able to display a non-zero win rate on this challenge. The tested methods were also unsuccessful in solving the \texttt{6h\_vs\_8z} scenario, which requires a fine-grained focus-fire by the allied Hydralisks. 

\texttt{MMM2} and \texttt{3s5z\_vs\_3s6z} are the harder asymmetric counterparts to \texttt{MMM} and \texttt{3s5z} respectively. Since the allied army is outnumbered by the enemy army, winning the battle requires significantly more coordination and strategy than in the symmetric case. These scenarios are examples of open-problems and will require algorithmic innovation. We plan to release further scenarios in this category but will also open the challenge for community contributions of new scenarios, which can be created using the StarCraft II map editor. %

\subsection{Feed-forward Agent Network}\label{appendix:FF_agents}

Table \ref{tab:qmix_rnn_ff_agent_results} shows the final median win rate for the QMIX agents with RNN and feed-forward agent networks. Although the final performance is comparable for 3 of the scenarios, the speed of learning can be quite different as shown in Figure \ref{fig:ff_graphs}. On the \texttt{2m\_vs\_1z} scenario, only the agents with RNNs are able to learn a good strategy.

\begin{table}[h]
	\centering
	\caption{Median win rate of QMIX with RNN vs QMIX with feed-forward agents across 12 seeds.}
	\begin{tabular}{ccccc}
		\toprule
		Scenario & RNN Agents & FF Agents \\
		\midrule
		\texttt{2s\_vs\_1sc} & 100 & 10  \\
		\texttt{3s\_vs\_3z} & 100  & 85  \\
		\texttt{so\_many\_banelings} & 100  & 100  \\
		\bottomrule
	\end{tabular}
	\label{tab:qmix_rnn_ff_agent_results}
\end{table}

\begin{figure}
	\centering
	\includegraphics[width=0.49\linewidth]{figures/graphs/3s_vs_3z_test_battle_won_mean_median_ff.png}
	\includegraphics[width=0.49\linewidth]{figures/graphs/micro_retarget_test_battle_won_mean_median_ff.png}
	\captionof{figure}{Median win rate of QMIX with RNN vs QMIX with feed-forward agents. 25\%-75\% percentile is shaded.}
	\label{fig:ff_graphs}
	\centering
\end{figure}
